# Supplementary material for: Improving dermatology classifiers across populations using images generated by large diffusion models
Source: arXiv:2211.13352 source file (2022-11-23)
Supplement: Supplementary file 1 [file supplementary_materials.tex]

% Supplementary Figure 1
% Un-selected images

% Supplementary Table 1
% Model accuracies on all skin conditions

% Supplementary Table 2
% Text prompts 
